# Supplementary material for: Investigating Non-local Features for Neural Constituency Parsing
Source: arXiv:2109.12814 source file (2022-03-28)
Supplement: Supplementary file 1 [file appendix.tex]

\appendix
\clearpage

\section{Detailed Experiment Settings}

\subsection{Dataset Statistics}
The statistics of PTB and CTB datasets are listed in Table~\ref{tab:data_statistics}. 
In particular, raw data for CTB is obtained from~\url{https://catalog.ldc.upenn.edu/LDC2005T01} and then pre-processed by the script released by ~\citet{san-constituency}~\footnote{Available at~\url{https://github.com/nikitakit/self-attentive-parser/tree/master/data/ctb_5.1}. }.

\begin{table}[h!]
    % \fontsize{10}{12}\selectfont
    \centering
    \begin{tabular}{c|ccc}
    \hline
    Data & \# Train & \# Dev & \# Test \\
    \hline
    PTB & 39,832 & 1,700 & 2,416 \\
    CTB & 17,544 & 352 & 348 \\
    \hline
    \end{tabular}
    \caption{Dataset statistics. \# indicates the number of sentences in the corresponding data split. }
    \label{tab:data_statistics}
\end{table}

\subsection{Implementation Details}

Our code is based on the open-sourced code~\footnote{Available at~\url{https://github.com/nikitakit/self-attentive-parser}.} of~\citet{san-constituency}. 
The training process gets terminated if no improvement on development F1 is obtained in the last 60 epochs. 
We evaluate the models which have the best F1 on the development set. 

For PTB, our method takes about 19 hours to train using PyTorch with a single RTX 2080Ti, while the baseline takes about 13 hours. 
For CTB, the approximate training time is 12 hours for ours and 7 hours for the baseline.
Our inference time is the same as that of the baseline parser, since no further computational operations are added to the inference phase. 
% Both are able to parse 219.6 sentences per second on the PTB test set. 
Both take about 11 seconds to parse the PTB section 23 (2416 sentences, an average of 23.5 tokens per sentence). 

The number of parameters is about 343.1 M for our PTB model with {\tt bert-large-uncased} and 104.1 M for our CTB model with {\tt bert-base-chinese}~\footnote{Both are downloaded from~\url{https://github.com/google-research/bert}.}. In comparison, the baseline parsers contain around 342.5 M parameters for PTB and 103.6 M parameters for CTB. 

Most of our hyperparameters are adopted from the baseline released code. 
% We further optimize the parameters with grid search: training batch size $\{32,64,128\}$ and scales of additional loss $\{1.0, 5.0, 10.0\}$.
For scales of the two additional losses, we set the scale of pattern loss to 1.0 and the scale of consistency loss to 5.0 for all experiments. 

To reduce the model size, we filter out those non-local pattern features that appear less than 5 times in the PTB training set and  those that account for less than 0.5\% of all pattern occurrences in the CTB training set. 
This results in moderate pattern vocabulary sizes of 841 for PTB and 514 for CTB. 

Following previous work, we use the EVALB~\footnote{Available at~\url{https://nlp.cs.nyu.edu/evalb/}.} script for evaluation. 
We evaluate with {\tt nk.prm} file~\footnote{Available at~\url{https://github.com/nikitakit/self-attentive-parser/blob/master/EVALB/nk.prm}.} that is released by~\citet{san-constituency}. 
We set {\tt DEBUG} option to 0 for all experiments except for drawing Figure~\ref{fig:span_length}, which requires detailed bracketing information by setting {\tt DEBUG} option to 2.

\label{sec:appendix}
